# Supplementary material for: Phase separation kinetics of 2-TIPS at low density: Cluster growth by ballistic agglomeration
Source: arXiv:2512.18615 source file (2025-12-21)
Supplement: Supplementary file 1 [file Lowdensity_kinetics_SM_dec21.pdf]

# Supplemental Material (SM)
# Phase separation kinetics of 2-TIPS at low density: Cluster growth by ballistic agglomeration

Nayana Venkatareddy[1], Partha Sarathi Mondal[2], Shradha Mishra[2], and Prabal K. Maiti[1]

[1]*Department of Physics, Indian Institute of Science, C. V. Raman Ave, Bengaluru 560012, India*
[2]*Department of Physics, Indian Institute of Technology (BHU), Varanasi, Uttar Pradesh 221005, India*

December 21, 2025

## 1 Molecular dynamics (MD) simulation details

We investigate the phase separation kinetics of two-temperature induced phase separation (2-TIPS) in a binary mixture of hot and cold particles using molecular dynamics (MD) simulations in two dimensions ($d$) at low density. The system consists of $N = 80,000$ particles, equally divided between hot and cold species, confined within $2d$ periodic simulation box. The particles interact via the Lennard-Jones (LJ) potential described in equation 1 of the main text. All MD simulation results are reported in reduced LJ units, where we take $\sigma$, $\epsilon$, and mass $m$ of the particles as fundamental units of length, energy, and mass, respectively. Hence, the density and temperature in reduced units are given by $\rho^* = \rho\sigma^2$ and $T^* = k_{\mathrm{B}}T/\epsilon$, respectively.

The simulations were performed in the NVT ensemble using the LAMMPS [1] software. To introduce the two-temperature model, we assign half of the particles in the system to the cold thermostat and the remaining half to the hot thermostat. We use Nosé-Hoover thermostat [2] to maintain the temperature of both hot ($T_h^*$) and cold ($T_c^*$) particles. The time step of integration is $\Delta t^* = 0.0005$, and the damping factor of the thermostat is chosen as $\tau_{\mathrm{T}} = 50 \times \Delta t^*$ as used in our previous works [3, 4]. All the simulations in the present work are carried out at a low density of $\rho^* = 0.1$.

Our previous studies have demonstrated [3, 4] that hot and cold particles undergo macroscopic phase separation when the temperature of hot particles is equal to or exceeds $T_h^* = 25$ at the density of $\rho^* = 0.1$. To investigate the kinetics of 2-TIPS, we first prepare the binary mixture in a homogeneous state by setting the temperatures of both hot ($T_h^*$) and cold ($T_c^*$) particles to $T^* = 2$. The system is equilibrated under these conditions for 4 million (M) time steps to ensure complete mixing. Subsequently, the system is quenched from this mixed state to a phase-separated state by instantaneously increasing the temperature of the hot particles to $T_h^* = 25$. We also perform an additional quench at $T_h^* = 40$. Following each quench, the simulations are carried out for 10M time steps, during which we analyze and quantify the temporal evolution of the domain morphologies as the system evolves from a homogeneous state to a phase-separated non-equilibrium steady state. All the dynamic quantities presented here are averaged over 10 independent runs to ensure a good statistical estimate.

## 2 Order parameter field from MD simulations

To quantify the structural characteristics of the evolving domain morphologies, an order parameter field must be defined that can distinguish between the phase-separating hot and cold regions. As discussed in the main text, the cold particles form denser regions compared to the hot particles. Therefore, we employ the local density differences between these regions to differentiate the two domains. Following the same procedure as in our previous work [5], we define a local density field $\rho(r, t)$, by mapping the particle positions in the simulation domain onto a lattice with spacing $\sigma$ (the diameter of a Lennard-Jones particle). The local density at each lattice site is then computed by counting the number of nearest neighbors.

In our earlier study [5] at high overall density ($\rho^* = 0.8$), the cold (hot) regions were identified as those where the local density was greater (less) than the overall average density. However, at the present lower overall density

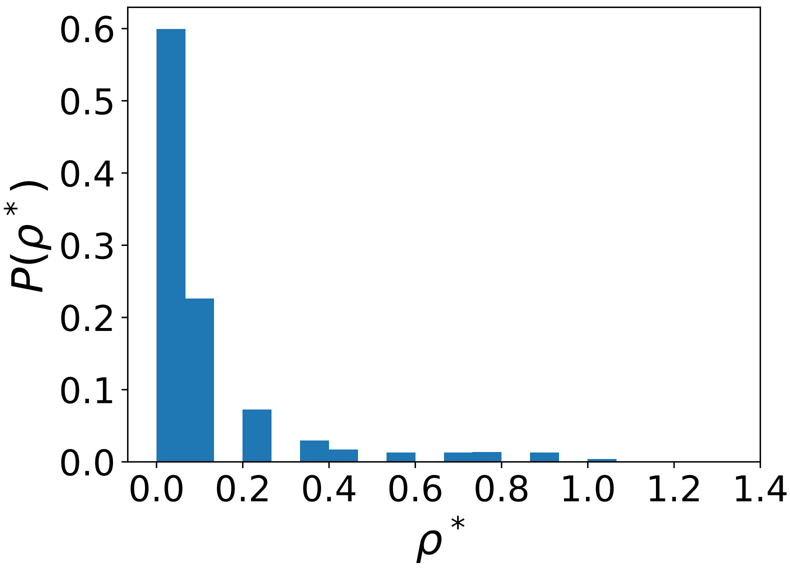


Figure 1: The figure depicts the histogram representing the probability distribution of the local density $P(\rho^*)$ of phase separating binary mixture of hot and cold particles at low overall density $\rho^* = 0.1$, at time $t = 2 \times 10^6$.

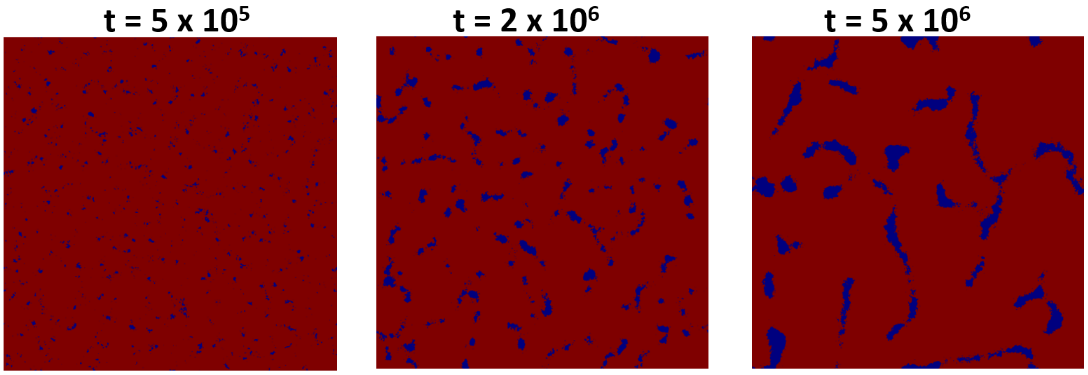


Figure 2: The temporal evolution of the order parameter field in MD simulations. The figure shows order parameter field $\phi(r,t)$ for quench temperature $T_h^* = 25$ and density $\rho^* = 0.1$, at various instants of time t. The cold particle rich regions with high density ($\rho^*(r) > 0.5$) are assigned $\phi(r) = 1$ and are depicted in dark blue color, while hot particle-rich regions with low density ($\rho^*(r) <= 0.5$) are assigned $\phi(r) = -1$ and are represented by dark red color.

($\rho^* = 0.1$), since the local density field $\rho(r,t)$ is evaluated by considering only the nearest neighbors on the lattice, the lowest non-zero density obtained is $\rho^* = 1/9 = 0.11$, which already exceeds the global average density. As a result, the above-described density criterion cannot be used to distinguish hot and cold phase-separating regions. The histogram of local density distribution $P(\rho^*)$ at time $t = 2 \times 10^6$ for the global density of $\rho^* = 0.1$ is illustrated in Fig. 1. The height of the distribution decreases with increasing density and becomes nearly constant for $\rho^* \geq 0.4$. Based on this, lattice sites with a majority of occupied neighboring sites (five or more out of nine) are classified as cold regions, and the rest as hot regions. Consequently, from the local density field $\rho(r,t)$, hardened order parameter field $\phi(r,t)$ is obtained by assigning $\phi = 1$ to dense cold regions ($\rho(r) > 0.5$) and $\phi = -1$ to dilute hot regions ($\rho(r) <= 0.5$). The order parameter field $\phi(r,t)$ for quench temperature $T_h^* = 25$ and density $\rho^* = 0.1$, at various instants of time, is illustrated in Fig. 2. The order parameter field clearly differentiates the cold clusters (blue color) from the surrounding dilute hot regions (red color).

## 3 Theory of ballistic agglomeration

Given that the phase-separating cold clusters exhibit ballistic motion before undergoing coalescence (Fig. 3(a) in main text), we compare our simulation results with the theoretical predictions of the ballistic agglomeration theory

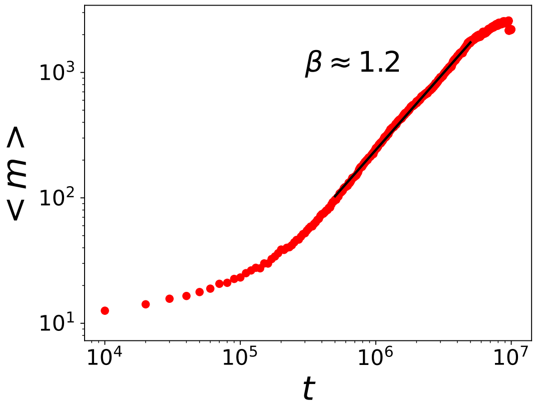


Figure 3: Plot of average mass of 20 largest clusters $< m >$ versus time for $T_h^* = 25$. The associated mass growth exponent ($m \sim t^{\beta}$) is $\beta \approx 1.2$ which agrees closely with $\beta_{theory} \approx 1.16$

described below.

Consider a system in $d$ dimensional space with $N$ clusters moving ballistically with an average root mean square (rms) velocity $v$. Let $n$ be the number density of clusters and $m$ be the average mass of clusters at a given time $t$. Assuming the clusters to be non-spherical in shape, the size of the clusters is characterized by their radius of gyration $R_g$, also a measure of collision cross-section. The average mass of clusters $m$ evolves with time as given in the equation below.

$$\frac{dm}{dt} = \frac{m}{\tau} \tag{1}$$

where $\tau = \frac{1}{nvR_g^{d-1}}$ (ratio of average volume per cluster to the rate of volume swept by the cluster) is the average time of collision between two clusters. We rewrite $n$, $v$ and $R_g$ in terms of average mass $m$, as $n \sim m^{-1}$, $v \sim m^{-z'}$ and $m \sim R_g^{d_f}$ respectively. Here $z'$ and fractal dimension $d_f$ are the exponents associated with mass dependence on velocity $v$ and radius of gyration $R_g$, respectively. Substituting them in equation 1, we obtain the solution

$$m \sim t^{\beta}, \beta = \frac{d_f}{d_f(1+z') - (d-1)} \tag{2}$$

To obtain the value of theoretical mass growth exponent $\beta_{theory}$ for low density kinetics in 2-TIPS, we calculate the value of fractal dimension $d_f$ and exponent $z'$ for phase separating cold clusters undergoing 2-TIPS. Using cluster analysis, we track the mass $m$, radius of gyration $R_g$, and rms velocity of centre of mass (cm) of the cold clusters $v$ as a function of time. It is important to note that, during cluster analysis, the hot particles trapped within the cold clusters are also considered as part of the cluster. Figures 3(b) and (c) in the main text illustrate the dependence of the radius of gyration $R_g$ and velocity $v$ of the cold clusters on mass $m$ of the clusters, respectively, for quench temperature $T_h^* = 25$. From the plot in Fig. 3(b) from main text, we obtain the fractal dimension $d_f$ of the cold clusters to be equal to $\approx 1.7$ ($< d = 2$), indicating the deviation from circular structure (typical in phase separating liquids). The value of exponent $z'$ extracted from plot in Fig. 3(c) in the main text, is $\approx 0.45$. Using these exponents, we get value of $\beta_{theory} \approx 1.16$, which inturn gives value of domain growth exponent $1/z_{theory} = \beta_{theory}/d_f \approx 0.68$. This theoretical value of $1/z_{theory}$ is in good agreement with the value of $1/z \approx 0.71$ (Fig. 2(b) in main text), obtained from the spatial correlation function $C_{\phi}(r,t)$, thus establishing cluster coalescence by ballistic agglomeration as the primary mechanism of 2-TIPS kinetics in low density. Further, the plot of average mass of the twenty largest clusters $< m >$ versus time in Fig. 3, gives $\beta \approx 1.2$, which is also consistent with the value of $\beta_{theory} \approx 1.16$.

# 4 MD results for quench temperature $T_h^* = 40$

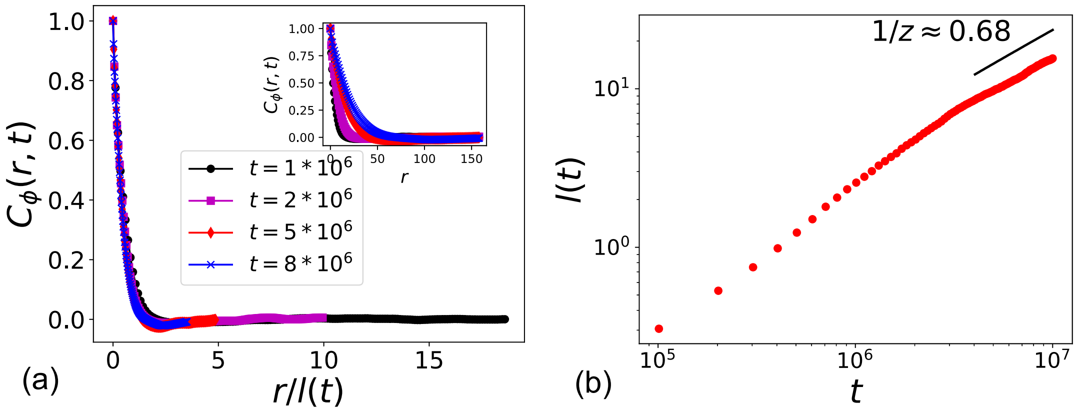


Figure 4: (a) Plot of the correlation function $C_\phi(r,t)$ as function of rescaled distance $r/l$, where $l$ is the characteristic length at density $\rho^* = 0.1$ for $T_h^* = 40$ at different instants of time. Inset illustrates plot of two-point spatial correlation function of $\phi$, $C_\phi(r,t)$ as function of distance between the points $r$ at density $\rho^* = 0.1$ for $T_h^* = 40$ at different instants of time. The correlation function $C_\phi(r,t)$ exhibits dynamic scaling. (b) Log-Log plot of characteristic length $l(t)$ versus time $t$ shows algebraic growth of $l(t)$. We see that the growth exponent $1/z$ has a value close to 0.68 at late times.

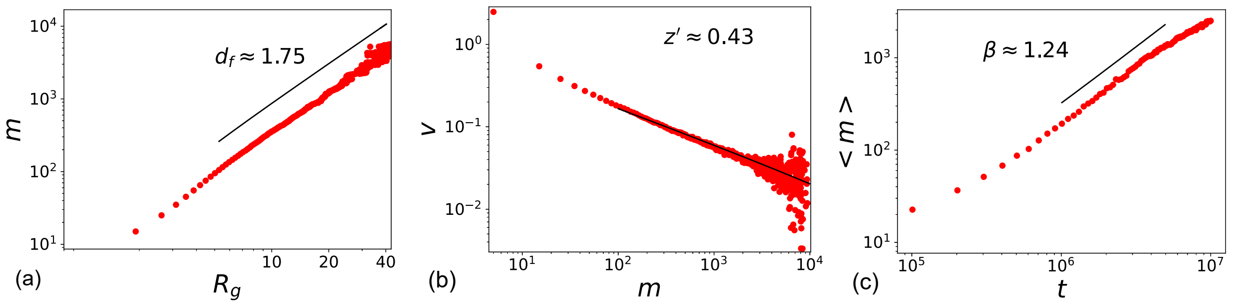


Figure 5: (a) Log-log plot of average mass $m$ of clusters versus average radius of gyration $R_g$ for $T_h^* = 40$. The power law exponent associated ($m \sim R_g^{d_f}$) with is $d_f \approx 1.75$. (b) Log-log plot of average rms velocity of clusters $v$ versus average mass $m$. The associated power law decay exponent ($v \sim m^{-z'}$) is $z' \approx 0.43$. (c) Plot of average mass of 20 largest clusters $< m >$ versus time. The associated mass growth exponent ($m \sim t^\beta$) is $\beta = 1.24$.

The results for quench temperature $T_h^* = 40$ and density $\rho^* = 0.1$ are presented in Figs. 4 and 5. Figure 4(a) shows the plot of correlation function $C_\phi(r,t)$ as a function of rescaled distance $r/l(t)$ (inset depicts $C_\phi(r,t)$ as a function of distance $r$) for $T_h^* = 40$. We see that correlation functions at different intervals of time converge onto a master plot, thus demonstrating dynamic scaling. Figure 4(b) illustrates the power law growth of characteristic length $l(t) \sim t^{1/z}$, with associated growth exponent $1/z \approx 0.68$. Figures 5(a) and (b) demonstrate the scaling relation between average mass of the cold clusters with their radius of gyration ($m \sim R_g^{d_f}$) and their rms velocity ($v \sim m^{-z'}$), respectively. From the plots we obtain the value of exponents $d_f \approx 1.75$ and $z' \approx 0.43$, which are also close to the exponents obtained for $T_h^* = 25$.

Substituting these values in equation 2, we obtain $\beta_{theory} \approx 1.17$, which yields $1/z_{theory} = \beta_{theory}/d_f \approx 0.66$. This value is close to $1/z = 0.68$ extracted from growth of characteristic length $l(t)$ (Fig 4(b)). Also, the cluster mass growth exponent $\beta \approx 1.24$ calculated from the plot of average mass of 20 largest clusters $< m >$, in Fig. 5(c), also closely matches with $\beta_{theory}$. These results further reinforce that ballistic agglomeration is the primary mechanism governing phase separation kinetics in 2-TIPS at low density.

# 5 Details of the coarse grained model

In a system of particles, the dynamics of the particles in a medium are governed by the interparticle interactions as well as the inertia. Hence, the momentum is a dynamical variable, and the state of the system is described by the position

and momentum of each particle. However, at the mesoscopic level, the dynamics of the same system is described by the time evolution of slow variables. On going from microscopic to mesoscopic scale, the selection of the slow variables is dictated by the conservation laws. Since the number of particles in the system is conserved, the local density field, $\rho(\boldsymbol{r})$, is a slow variable. On the other hand, if the surrounding medium is low viscous, then the momentum relaxes on a time scale which is much larger than the microscopic time scales. Thus, momentum density, $\boldsymbol{g}(\boldsymbol{r})$, is a slow variable in such systems and the dynamics of the resulting velocity field, $\boldsymbol{u}(\boldsymbol{r}) = \frac{\boldsymbol{g}}{\rho}$ is described by the Navier Stokes Equation (NSE).

In case of a mixture of two species at different temperatures, it is observed that the one with lower temperature form dense domains, resulting in a temperature difference between the interior and exterior of the domains. The gradient of temperature across the interface, results in additional nonequilibrium stress. Thus, the stress in NSE can be decomposed in two parts, $\boldsymbol{\Sigma} = \boldsymbol{\Sigma}_p + \boldsymbol{\Sigma}_a$, where $\boldsymbol{\Sigma}_p$ is the passive component of stress which emerges due to the density gradient at the interface. $\boldsymbol{\Sigma}_a$ is called the active stress since it originates from the temperature difference across the interface.

For the conserved order parameter corresponding to the density field of hot and cold species, $\psi_{\mathrm{h}}$ and $\psi_{\mathrm{c}}$, the dynamics can be described in terms of Free energy functional, $\mathcal{F}_{mix} = \mathcal{F}_{\mathrm{c}} + \mathcal{F}_{\mathrm{h}}$ where,

$$\mathcal{F}_{\mathrm{c}}[\psi_{\mathrm{c,h}}(\boldsymbol{r},t)] = \int \left\{ \frac{\alpha_{\mathrm{c}}}{2}\psi_{\mathrm{c}}^2 + \frac{\beta_{\mathrm{c}}}{4}\psi_{\mathrm{c}}^4 + \frac{\kappa_{\mathrm{c}}}{2}(\nabla\psi_{\mathrm{c}})^2 + \frac{\gamma_{\mathrm{c}}}{2}\psi_{\mathrm{c}}^2\psi_{\mathrm{h}} \right\} d^D r$$

and

$$\mathcal{F}_{\mathrm{h}}[\psi_{\mathrm{c,h}}(\boldsymbol{r},t)] = \int \left\{ \frac{\alpha_{\mathrm{h}}}{2}\psi_{\mathrm{h}}^2 + \frac{\beta_{\mathrm{h}}}{4}\psi_{\mathrm{h}}^4 + \frac{\kappa_{\mathrm{h}}}{2}(\nabla\psi_{\mathrm{h}})^2 - \frac{\gamma_{\mathrm{h}}}{2}\psi_{\mathrm{h}}^2\psi_{\mathrm{c}} \right\} d^D r$$

In $\mathcal{F}_{\mathrm{c}}$ and $\mathcal{F}_{\mathrm{h}}$, the first three terms in the integrand describe the self-interaction of each species, and the last two terms are the coupling terms accounting for the inter-species interaction. The coupling terms are motivated by the fact that inter-species interactions effectively reduce the temperature of the hot particles and increase that of the cold particles. The dynamical equations are given by,

$$D_t\psi_{\mathrm{c}}(\mathbf{r},t) = \nabla^2\left(\frac{\delta\mathcal{F}_{\mathrm{mix}}}{\delta\psi_{\mathrm{c}}}\right) = \nabla^2\Big[\alpha_{\mathrm{c}}\,\psi_{\mathrm{c}} + \beta_{\mathrm{c}}\,\psi_{\mathrm{c}}^3 - \kappa_{\mathrm{c}}\,\nabla^2\psi_{\mathrm{c}} + \gamma_{\mathrm{c}}\,\psi_{\mathrm{h}}\,\psi_{\mathrm{c}} - \tfrac{\gamma_{\mathrm{h}}}{2}\,\psi_{\mathrm{h}}^2\Big]$$

$$D_t\psi_{\mathrm{h}}(\mathbf{r},t) = \nabla^2\left(\frac{\delta\mathcal{F}_{\mathrm{mix}}}{\delta\psi_{\mathrm{h}}}\right) = \nabla^2\Big[\alpha_{\mathrm{h}}\,\psi_{\mathrm{h}} + \beta_{\mathrm{h}}\,\psi_{\mathrm{h}}^3 - \kappa_{\mathrm{h}}\,\nabla^2\psi_{\mathrm{h}} - \gamma_{\mathrm{h}}\,\psi_{\mathrm{c}}\,\psi_{\mathrm{h}} + \tfrac{\gamma_{\mathrm{c}}}{2}\,\psi_{\mathrm{c}}^2\Big]$$

where, $D_t = \partial_t + \gamma(\boldsymbol{u}.\boldsymbol{\nabla})$ denotes the material derivative.

# 6 Simulation details of the coarse grained model

The coarse-grained model is simulated in a $2d$ square box of size $L$ with periodic boundary conditions along both directions. Eqs.(3-5) in the main manuscript are simulated using a Finite Time Central Space (FTCS) integration scheme with spatial and temporal grid size $\Delta X$ and $\Delta t$, respectively, satisfying the criteria $\frac{\Delta t}{(\Delta X)^2} < \frac{1}{2}$ for numerical stability. In our simulation, we set $\Delta X = 1.0$ and $\Delta t = 0.01$. The results presented in the article correspond to system size $L = 1024$, for which the system is simulated for $10^6$ time steps. One simulation step is counted when the state of the system (i.e. $\{\psi_{\mathrm{c}}, \psi_{\mathrm{h}}, \boldsymbol{u}\}$) is updated once. For better statistics, data (except snapshots) are averaged over 100 independent realizations.
The average value of the density order parameter for the cold and hot species can be defined as $\psi_{0,c/h} = \frac{1}{L^2}\sum_{\boldsymbol{r}}\psi_{c/h}(\boldsymbol{r})$. The mean density of the cold and hot species can be approximately calculated as $\rho_{0,c/h} \approx \frac{1+\psi_{0,c/h}}{2}$. The mean density of the system, $\rho_0$, is given by $\rho_0 = \rho_{0,c} + \rho_{0,h}$. $\psi_{0,c/h} \approx 0$ represents a densely packed system of cold and hot particles, with $\psi_{0,c/h} < 0$ indicating a decrease in overall density. The mixture is symmetric when $\psi_{0,c} = \psi_{0,h}$ and asymmetric otherwise. Initially, at each lattice point $\psi_{c/h}$ are distributed uniformly in the interval $[-\xi, \xi]$ around $\psi_{0,c/h}$, where $\xi = 0.05$. Different independent realizations correspond to distinct seeds of the random number generator.

# 7 Growth Kinetics

In this section, we present some additional results on the growth kinetics of 2-TIPS at low density. Fig. 6(a) shows the time evolution of the characteristic length scale, $l(t)$, for two different activity, $\chi = 2.10$ and $2.20$, at a fixed density

$\rho_0 \approx 0.40$. In both cases, the domain growth follows a power-law behavior, $\approx t^{0.70}$. Further, Fig. 6(b) displays the scaling collapse of the correlation function when plotted with scaled distance $r/l$ for $\rho_0 \approx 0.30$ and $\chi = 2.20$. Together with Fig. 4(c) of the main text, these results confirm the existence of a dynamic scaling regime during the coarsening process in the low-density regime.

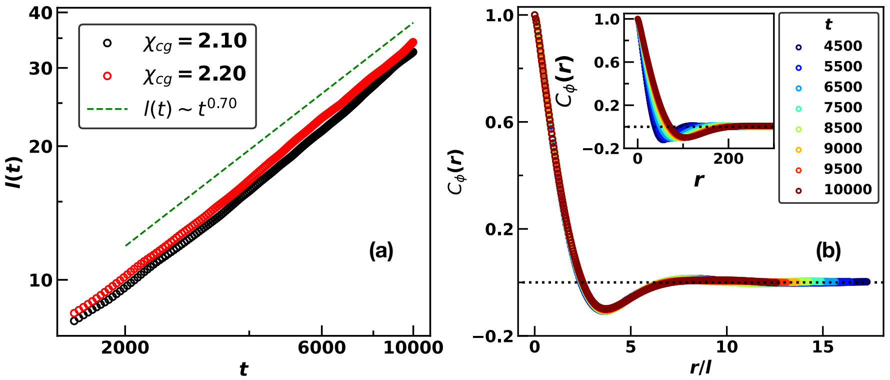


Figure 6: Panel (a) shows the plot of time dependent domain size $l(t)$ *vs.* $t$ on log-log scale for two different activity for $\rho_0 \approx 0.40$; Panel (b) shows the plot of scaled correlation function $C(r)$ *vs.* scaled distance $r/l$ at different times collapses onto a master curve for $\rho_0 \approx 0.30$ and $\chi_{cg} = 2.20$. (Inset) Plot of the unscaled correlation function, $C(r)$ *vs* $r$.

# 8 Description of the supplementary movies

**MOVIE-1: Kinetics of phase separation in 2-TIPS at low density from MD simulations**

The supplementary movie depicts the phase separation kinetics in 2-TIPS at low density, in a symmetric binary mixture of hot (red) and cold (blue) particles. After the quench, cold nuclei nucleate within a sea of hot particles. These cold clusters then migrate and merge with others, progressively forming larger phase-separated structures. The ballistic motion of the clusters toward one another indicates an effective attractive interaction driving the coalescence process.

*Parameters*: System size $N = 80,000$, quench temperature $T_h^* = 25$, density $\rho^* = 0.1$.

*Link* : `https://1drv.ms/v/c/fa311ca96e9b7429/EVxB5_RVkFJGje7rspkXhlsBg7C8u3zzKC5WgYK78bL1kA?e=z1xQo6`

**MOVIE-2 : Ballistic motion of few cold clusters from MD simulation**

The supplementary movie provides a magnified view of MOVIE-1, wherein the ballistic migration of cold clusters toward each other becomes evident.

*Parameters* : System size $N = 80,000$, quench temperature $T_h^* = 25$ , density $\rho^* = 0.1$.

*Link* : `https://1drv.ms/i/c/fa311ca96e9b7429/Ect3qOCp3dtMto8p4naAaQQBnJm7_5nOljQDQEXrAzQm2g?e=Snu9ct`

**MOVIE-3 : Emergence of phase separation in the coarse grained model**

The supplementary movie shows the emergence of phase separation between cold and hot particles in the mixture starting from a homogeneously mixed state. The heatmap depicts the local phase-separation order parameter, defined as $\phi(\boldsymbol{r}, t) = \psi_{\rm h}(\boldsymbol{r}, t) - \psi_{\rm c}(\boldsymbol{r}, t)$, with the corresponding values indicated by the colorbar. Regions where $\phi < 0$ ($\phi > 0$) correspond to the cold (hot) majority domains. The movie clearly shows the emergence of cold droplets through nucleation events.

*Parameters* : System size $L = 512$, activity $\chi = 2.20$, off-criticality $\psi_0 = -0.60$ ($\rho_0 = 0.40$).

*Link* : `https://drive.google.com/file/d/187oGptGxhfTZfdAQN1xrcc4FPSrsKZKh/view?usp=sharing`

**MOVIE-4 : Droplet coalescence in coarse grained model**

The supplementary movie illustrates the coarsening dynamics of the $\phi$ field via droplet coalescence, focusing onto a subregion of the entire simulation box. The movie clearly shows that the small droplet shows significant translational dynamics, whereas larger droplets remain largely immobile while exhibiting shape modulations either due to dynamics of larger droplets in its vicinity or before the coalescence events. The details of the heatmap are the same as in MOVIE-3.

*Parameters* : System size $L = 512$ (zoomed into a $250 \times 250$ box in the system), activity $\chi = 2.20$, off-criticality

$\psi_0 = -0.60$ ($\rho_0 = 0.40$).
*Link* : `https://drive.google.com/file/d/1WCD1mEkZFhDqLyq3CnJbXQk-EhpLAluc/view?usp=sharing`

**MOVIE-5 : Droplet dynamics in coarse grained model**
This supplementary movie highlights the droplet dynamics by focusing on a single droplet within the system. The details of the heatmap is same as in MOVIE-3.
*Parameters* : System size $L = 512$, activity $\chi = 2.20$, off-criticality $\psi_0 = -0.60$ ($\rho_0 = 0.40$).
*Link* : `https://drive.google.com/file/d/1BcYFwDeWR7hplTAsJay_QmUIcnJLc-Cx/view?usp=sharing`

# References


[1] A. P. Thompson, H. M. Aktulga, R. Berger, D. S. Bolintineanu, W. M. Brown, P. S. Crozier, P. J. in 't Veld, A. Kohlmeyer, S. G. Moore, T. D. Nguyen, R. Shan, M. J. Stevens, J. Tranchida, C. Trott, and S. J. Plimpton. LAMMPS - a flexible simulation tool for particle-based materials modeling at the atomic, meso, and continuum scales. *Comp. Phys. Comm.*, 271:108171, 2022.

[2] Denis J Evans and Brad Lee Holian. The nose–hoover thermostat. *The Journal of chemical physics*, 83(8):4069–4074, 1985.

[3] S Siva Nasarayya Chari, Chandan Dasgupta, and Prabal K Maiti. Scalar activity induced phase separation and liquid–solid transition in a lennard-jones system. *Soft matter*, 15(36):7275–7285, 2019.

[4] Nayana Venkatareddy, Jaydeep Mandal, and Prabal K. Maiti. Effect of confinement and topology: 2-tips vs. mips. *Soft Matter*, 19:8561–8576, 2023.

[5] Nayana Venkatareddy, Partha Sarathi Mondal, Jaydeep Mandal, Shradha Mishra, and Prabal K. Maiti. Growth laws and universality in two-temperature induced phase separation: Microscopic and coarse-grained approach. *Phys. Rev. E*, 112:015409, Jul 2025.
